# Supplementary material for: 3D Multi-View Stylization with Pose-Free Correspondences Matching for Robust 3D Geometry Preservation
Source: arXiv:2604.09639 source file (2026-03-22)
Supplement: Supplementary file 1 [file appendix.tex]

\chapter{General Addenda}

If there are several additions you want to add, but they do not fit into the thesis itself, they belong here.

\section{Detailed Addition}

Even sections are possible, but usually only used for several elements in, e.g.\ tables, images, etc.

\chapter{Figures}
\section{Example 1}
\cmark
\section{Example 2}
\xmark
